# Supplementary material for: Studying excited-state-specific perturbation theory on the Thiel set
Source: arXiv:2302.07240 source file (2023-05-20)
Supplement: Supplementary file 1 [file acetamide_vs_TBE_errors_w_amps.tex]

\begin{table}[htp]
\caption{ 
\label{tab:acetamide_ESMP2_vs_TBE_amps}
Absolute ESMF, ESMP2 and level shifted ESMP2 (level shift = 0.50 a.u.) errors vs. the Thiel best estimates (TBEs) and the corresponding norm of the doubles amplitudes calculated from the norm of the first order ESMP wave function for acetamide.}
\begin{tabular}{l | c c | c c}
\hline\hline
\hspace{2mm} State & 
\hspace{2mm} lvl=0.0 error & 
\hspace{2mm} norm  & 
\hspace{2mm} lvl=0.5 error & 
\hspace{2mm} norm  
\\[2pt] 
\hline 
\hspace{0.0mm} $1^1A^{\prime\prime}$ & 0.14 & 0.18 & 0.27 & 0.14 \\ 
\hspace{0.0mm} $2^1A'$ & 0.39 & 0.27 & 0.03 & 0.20 \\ 
\hline\hline 
\end{tabular} 
\end{table}
