# Supplementary material for: Studying excited-state-specific perturbation theory on the Thiel set
Source: arXiv:2302.07240 source file (2023-05-20)
Supplement: Supplementary file 8 [file cyclopropene_vs_TBE_errors_w_amps.tex]

\begin{table}[htp]
\caption{ 
\label{tab:cyclopropene_ESMP2_vs_TBE_amps}
Absolute ESMF, ESMP2 and level shifted ESMP2 (level shift = 0.50 a.u.) errors vs. the Thiel best estimates (TBEs) and the corresponding norm of the doubles amplitudes calculated from the norm of the first order ESMP wave function for cyclopropene.}
\begin{tabular}{l | c c | c c}
\hline\hline
\hspace{2mm} State & 
\hspace{2mm} lvl=0.0 error & 
\hspace{2mm} norm & 
\hspace{2mm} lvl=0.5 error & 
\hspace{2mm} norm 
\\[2pt] 
\hline 
\hspace{0.0mm} $1^1B_{1}$ & 0.20 & 0.20 & 0.15 & 0.15 \\ 
\hspace{0.0mm} $1^1B_{2}$ & 0.31 & 0.20 & 0.21 & 0.15 \\ 
\hline\hline 
\end{tabular} 
\end{table}
