# Supplementary material for: Studying excited-state-specific perturbation theory on the Thiel set
Source: arXiv:2302.07240 source file (2023-05-20)
Supplement: Supplementary file 30 [file acetone_vs_TBE_errors.tex]

\begin{table}[htp]
\caption{ 
\label{tab:acetone_ESMP2_vs_TBE}
Absolute ESMF, ESMP2 and level shifted ESMP2 (level shift = 0.50 a.u.) results vs. the Thiel best estimates (TBEs) for acetone.}
\begin{tabular}{l| c | c c | c c | c c}
\hline\hline
\hspace{2mm} State & 
\hspace{2mm} TBE & 
\hspace{2mm} ESMF & 
\hspace{2mm} error & 
\hspace{2mm} ESMP2 & 
\hspace{2mm} error & 
\hspace{2mm} shift=0.50 a.u. & 
\hspace{2mm} error 
\\[2pt] 
\hline 
\hspace{0.0mm} $1^1A_{2}$ & 4.40 & 3.47 & 0.93 & 4.39 & 0.01 & 4.28 & 0.12 \\ 
\hspace{0.0mm} $1^1B_{1}$ & 9.10 & 8.48 & 0.62 & 9.22 & 0.12 & 9.16 & 0.06 \\ 
\hspace{0.0mm} $2^1A_{1}$ & 9.40 & 8.82 & 0.58 & 9.08 & 0.32 & 9.28 & 0.12 \\ 
\hline\hline 
\end{tabular} 
\end{table}
