# Supplementary material for: Studying excited-state-specific perturbation theory on the Thiel set
Source: arXiv:2302.07240 source file (2023-05-20)
Supplement: Supplementary file 31 [file adenine_vs_TBE_errors.tex]

\begin{table}[htp]
\caption{ 
\label{tab:adenine_ESMP2_vs_TBE}
Absolute ESMF, ESMP2 and level shifted ESMP2 (level shift = 0.50 a.u.) results vs. the Thiel best estimates (TBEs) for adenine.}
\begin{tabular}{l| c | c c | c c | c c}
\hline\hline
\hspace{2mm} State & 
\hspace{2mm} TBE & 
\hspace{2mm} ESMF & 
\hspace{2mm} error & 
\hspace{2mm} ESMP2 & 
\hspace{2mm} error & 
\hspace{2mm} shift=0.50 a.u. & 
\hspace{2mm} error 
\\[2pt] 
\hline 
\hspace{0.0mm} $2^1A'$ & 5.25 & 6.52 & 1.27 & 4.41 & 0.84 & 5.36 & 0.11 \\ 
\hspace{0.0mm} $3^1A'$ & 5.25 & 5.94 & 0.69 & 4.90 & 0.35 & 5.37 & 0.12 \\ 
\hspace{0.0mm} $1^1A^{\prime\prime}$ & 5.12 & 6.33 & 1.21 & 4.87 & 0.25 & 5.44 & 0.32 \\ 
\hspace{0.0mm} $2^1A^{\prime\prime}$ & 5.75 & 7.00 & 1.25 & 5.12 & 0.63 & 5.84 & 0.09 \\ 
\hline\hline 
\end{tabular} 
\end{table}
