# Supplementary material for: Studying excited-state-specific perturbation theory on the Thiel set
Source: arXiv:2302.07240 source file (2023-05-20)
Supplement: Supplementary file 32 [file benzene_vs_TBE_errors.tex]

\begin{table}[htp]
\caption{ 
\label{tab:benzene_ESMP2_vs_TBE}
Absolute ESMF, ESMP2 and level shifted ESMP2 (level shift = 0.50 a.u.) results vs. the Thiel best estimates (TBEs) for benzene.}
\begin{tabular}{l| c | c c | c c | c c}
\hline\hline
\hspace{2mm} State & 
\hspace{2mm} TBE & 
\hspace{2mm} ESMF & 
\hspace{2mm} error & 
\hspace{2mm} ESMP2 & 
\hspace{2mm} error & 
\hspace{2mm} shift=0.50 a.u. & 
\hspace{2mm} error 
\\[2pt] 
\hline 
\hspace{0.0mm} $1^1B_{2u}$ & 5.08 & 6.08 & 1.00 & 4.03 & 1.05 & 4.98 & 0.10 \\ 
\hspace{0.0mm} $1^1B_{1u}$ & 6.54 & 6.22 & 0.32 & 6.07 & 0.47 & 6.24 & 0.30 \\ 
\hspace{0.0mm} $1^1E_{1u}$ & 7.13 & 7.89 & 0.76 & 6.48 & 0.65 & 7.11 & 0.02 \\ 
\hspace{0.0mm} $2^1E_{2g}$ & 8.41 & 10.65 & 2.24 & 7.60 & 0.81 & 9.37 & 0.96 \\ 
\hline\hline 
\end{tabular} 
\end{table}
