# Supplementary material for: Studying excited-state-specific perturbation theory on the Thiel set
Source: arXiv:2302.07240 source file (2023-05-20)
Supplement: Supplementary file 33 [file benzoquinone_vs_TBE_errors.tex]

\begin{table}[htp]
\caption{ 
\label{tab:benzoquinone_ESMP2_vs_TBE}
Absolute ESMF, ESMP2 and level shifted ESMP2 (level shift = 0.50 a.u.) results vs. the Thiel best estimates (TBEs) for benzoquinone.}
\begin{tabular}{l| c | c c | c c | c c}
\hline\hline
\hspace{2mm} State & 
\hspace{2mm} TBE & 
\hspace{2mm} ESMF & 
\hspace{2mm} error & 
\hspace{2mm} ESMP2 & 
\hspace{2mm} error & 
\hspace{2mm} shift=0.50 a.u. & 
\hspace{2mm} error 
\\[2pt] 
\hline 
\hspace{0.0mm} $1^1A_{u}$ & 2.80 & 3.52 & 0.72 & 1.77 & 1.03 & 2.61 & 0.19 \\ 
\hspace{0.0mm} $1^1B_{1g}$ & 2.78 & 3.50 & 0.72 & 1.69 & 1.09 & 2.52 & 0.26 \\ 
\hspace{0.0mm} $1^1B_{3g}$ & 4.25 & 4.56 & 0.31 & 3.67 & 0.58 & 4.12 & 0.13 \\ 
\hspace{0.0mm} $1^1B_{1u}$ & 5.29 & 6.03 & 0.74 & 4.70 & 0.59 & 5.31 & 0.02 \\ 
\hspace{0.0mm} $1^1B_{3u}$ & 5.60 & 8.14 & 2.54 & 4.88 & 0.72 & 6.14 & 0.54 \\ 
\hspace{0.0mm} $2^1B_{3g}$ & 6.98 & 8.27 & 1.29 & 6.03 & 0.95 & 7.01 & 0.03 \\ 
\hline\hline 
\end{tabular} 
\end{table}
