# Supplementary material for: Studying excited-state-specific perturbation theory on the Thiel set
Source: arXiv:2302.07240 source file (2023-05-20)
Supplement: Supplementary file 34 [file butadiene_vs_TBE_errors.tex]

\begin{table}[htp]
\caption{ 
\label{tab:butadiene_ESMP2_vs_TBE}
Absolute ESMF, ESMP2 and level shifted ESMP2 (level shift = 0.50 a.u.) results vs. the Thiel best estimates (TBEs) for butadiene.}
\begin{tabular}{l| c | c c | c c | c c}
\hline\hline
\hspace{2mm} State & 
\hspace{2mm} TBE & 
\hspace{2mm} ESMF & 
\hspace{2mm} error & 
\hspace{2mm} ESMP2 & 
\hspace{2mm} error & 
\hspace{2mm} shift=0.50 a.u. & 
\hspace{2mm} error 
\\[2pt] 
\hline 
\hspace{0.0mm} $1^1B_{u}$ & 6.18 & 6.29 & 0.12 & 6.02 & 0.16 & 6.18 & 0.00 \\ 
\hspace{0.0mm} $2^1A_{g}$ & 6.55 & 8.85 & 2.30 & 4.31 & 2.24 & 6.98 & 0.43 \\ 
\hline\hline 
\end{tabular} 
\end{table}
