# Supplementary material for: Studying excited-state-specific perturbation theory on the Thiel set
Source: arXiv:2302.07240 source file (2023-05-20)
Supplement: Supplementary file 35 [file cyclopentadiene_vs_TBE_errors.tex]

\begin{table}[htp]
\caption{ 
\label{tab:cyclopentadiene_ESMP2_vs_TBE}
Absolute ESMF, ESMP2 and level shifted ESMP2 (level shift = 0.50 a.u.) results vs. the Thiel best estimates (TBEs) for cyclopentadiene.}
\begin{tabular}{l| c | c c | c c | c c}
\hline\hline
\hspace{2mm} State & 
\hspace{2mm} TBE & 
\hspace{2mm} ESMF & 
\hspace{2mm} error & 
\hspace{2mm} ESMP2 & 
\hspace{2mm} error & 
\hspace{2mm} shift=0.50 a.u. & 
\hspace{2mm} error 
\\[2pt] 
\hline 
\hspace{0.0mm} $1^1B_{2}$ & 5.55 & 5.40 & 0.15 & 5.23 & 0.32 & 5.36 & 0.19 \\ 
\hspace{0.0mm} $2^1A_{1}$ & 6.31 & 8.27 & 1.96 & 4.83 & 1.48 & 6.60 & 0.29 \\ 
\hline\hline 
\end{tabular} 
\end{table}
