# Supplementary material for: Studying excited-state-specific perturbation theory on the Thiel set
Source: arXiv:2302.07240 source file (2023-05-20)
Supplement: Supplementary file 39 [file formaldehyde_vs_TBE_errors.tex]

\begin{table}[htp]
\caption{ 
\label{tab:formaldehyde_ESMP2_vs_TBE}
Absolute ESMF, ESMP2 and level shifted ESMP2 (level shift = 0.50 a.u.) results vs. the Thiel best estimates (TBEs) for formaldehyde.}
\begin{tabular}{l| c | c c | c c | c c}
\hline\hline
\hspace{2mm} State & 
\hspace{2mm} TBE & 
\hspace{2mm} ESMF & 
\hspace{2mm} error & 
\hspace{2mm} ESMP2 & 
\hspace{2mm} error & 
\hspace{2mm} shift=0.50 a.u. & 
\hspace{2mm} error 
\\[2pt] 
\hline 
\hspace{0.0mm} $1^1A_{2}$ & 3.88 & 2.93 & 0.95 & 3.96 & 0.08 & 3.81 & 0.07 \\ 
\hspace{0.0mm} $1^1B_{1}$ & 9.10 & 8.12 & 0.98 & 9.12 & 0.02 & 8.98 & 0.12 \\ 
\hspace{0.0mm} $2^1A_{1}$ & 9.30 & 9.22 & 0.08 & 9.78 & 0.48 & 9.90 & 0.60 \\ 
\hline\hline 
\end{tabular} 
\end{table}
