# Supplementary material for: Studying excited-state-specific perturbation theory on the Thiel set
Source: arXiv:2302.07240 source file (2023-05-20)
Supplement: Supplementary file 40 [file formamide_vs_TBE_errors.tex]

\begin{table}[htp]
\caption{ 
\label{tab:formamide_ESMP2_vs_TBE}
Absolute ESMF, ESMP2 and level shifted ESMP2 (level shift = 0.50 a.u.) results vs. the Thiel best estimates (TBEs) for formamide.}
\begin{tabular}{l| c | c c | c c | c c}
\hline\hline
\hspace{2mm} State & 
\hspace{2mm} TBE & 
\hspace{2mm} ESMF & 
\hspace{2mm} error & 
\hspace{2mm} ESMP2 & 
\hspace{2mm} error & 
\hspace{2mm} shift=0.50 a.u. & 
\hspace{2mm} error 
\\[2pt] 
\hline 
\hspace{0.0mm} $1^1A^{\prime\prime}$ & 5.63 & 4.56 & 1.07 & 5.62 & 0.01 & 5.47 & 0.16 \\ 
\hspace{0.0mm} $2^1A'$ & 7.44 & 7.03 & 0.41 & 7.42 & 0.02 & 7.52 & 0.08 \\ 
\hline\hline 
\end{tabular} 
\end{table}
