# Supplementary material for: Studying excited-state-specific perturbation theory on the Thiel set
Source: arXiv:2302.07240 source file (2023-05-20)
Supplement: Supplementary file 43 [file imidazole_vs_TBE_errors.tex]

\begin{table}[htp]
\caption{ 
\label{tab:imidazole_ESMP2_vs_TBE}
Absolute ESMF, ESMP2 and level shifted ESMP2 (level shift = 0.50 a.u.) results vs. the Thiel best estimates (TBEs) for imidazole.}
\begin{tabular}{l| c | c c | c c | c c}
\hline\hline
\hspace{2mm} State & 
\hspace{2mm} TBE & 
\hspace{2mm} ESMF & 
\hspace{2mm} error & 
\hspace{2mm} ESMP2 & 
\hspace{2mm} error & 
\hspace{2mm} shift=0.50 a.u. & 
\hspace{2mm} error 
\\[2pt] 
\hline 
\hspace{0.0mm} $1^1A^{\prime\prime}$ & 6.81 & 6.11 & 0.70 & 6.80 & 0.01 & 6.72 & 0.09 \\ 
\hspace{0.0mm} $2^1A'$ & 6.19 & 7.08 & 0.89 & 5.65 & 0.54 & 6.49 & 0.30 \\ 
\hspace{0.0mm} $3^1A'$ & 6.93 & 7.77 & 0.84 & 7.01 & 0.08 & 7.36 & 0.43 \\ 
\hline\hline 
\end{tabular} 
\end{table}
