# Supplementary material for: Studying excited-state-specific perturbation theory on the Thiel set
Source: arXiv:2302.07240 source file (2023-05-20)
Supplement: Supplementary file 44 [file naphthalene_vs_TBE_errors.tex]

\begin{table}[htp]
\caption{ 
\label{tab:naphthalene_ESMP2_vs_TBE}
Absolute ESMF, ESMP2 and level shifted ESMP2 (level shift = 0.50 a.u.) results vs. the Thiel best estimates (TBEs) for naphthalene.}
\begin{tabular}{l| c | c c | c c | c c}
\hline\hline
\hspace{2mm} State & 
\hspace{2mm} TBE & 
\hspace{2mm} ESMF & 
\hspace{2mm} error & 
\hspace{2mm} ESMP2 & 
\hspace{2mm} error & 
\hspace{2mm} shift=0.50 a.u. & 
\hspace{2mm} error 
\\[2pt] 
\hline 
\hspace{0.0mm} $1^1B_{3u}$ & 4.24 & 5.17 & 0.93 & 3.22 & 1.02 & 4.13 & 0.11 \\ 
\hspace{0.0mm} $1^1B_{2u}$ & 4.77 & 5.04 & 0.27 & 4.33 & 0.44 & 4.73 & 0.04 \\ 
\hspace{0.0mm} $2^1A_{g}$ & 5.90 & 7.28 & 1.38 & 5.06 & 0.84 & 6.11 & 0.21 \\ 
\hspace{0.0mm} $1^1B_{1g}$ & 6.00 & 6.69 & 0.69 & 5.96 & 0.04 & 6.37 & 0.37 \\ 
\hspace{0.0mm} $2^1B_{3u}$ & 6.07 & 6.85 & 0.78 & 5.33 & 0.74 & 5.99 & 0.08 \\ 
\hspace{0.0mm} $2^1B_{1g}$ & 6.48 & 7.76 & 1.28 & 4.96 & 1.52 & 6.30 & 0.18 \\ 
\hspace{0.0mm} $2^1B_{2u}$ & 6.33 & 7.11 & 0.78 & 5.42 & 0.91 & 6.22 & 0.11 \\  
\hline\hline 
\end{tabular} 
\end{table}
