# Supplementary material for: Studying excited-state-specific perturbation theory on the Thiel set
Source: arXiv:2302.07240 source file (2023-05-20)
Supplement: Supplementary file 46 [file octatetraene_vs_TBE_errors.tex]

\begin{table}[htp]
\caption{ 
\label{tab:octatetraene_ESMP2_vs_TBE}
Absolute ESMF, ESMP2 and level shifted ESMP2 (level shift = 0.50 a.u.) results vs. the Thiel best estimates (TBEs) for octatetraene.}
\begin{tabular}{l| c | c c | c c | c c}
\hline\hline
\hspace{2mm} State & 
\hspace{2mm} TBE & 
\hspace{2mm} ESMF & 
\hspace{2mm} error & 
\hspace{2mm} ESMP2 & 
\hspace{2mm} error & 
\hspace{2mm} shift=0.50 a.u. & 
\hspace{2mm} error 
\\[2pt] 
\hline 
\hspace{0.0mm} $2^1A_{g}$ & 4.47 & 7.01 & 2.54 & 1.19 & 3.28 & 4.99 & 0.52 \\ 
\hspace{0.0mm} $1^1B_{u}$ & 4.66 & 4.71 & 0.05 & 4.16 & 0.50 & 4.43 & 0.23 \\ 
\hline\hline 
\end{tabular} 
\end{table}
