# Supplementary material for: Studying excited-state-specific perturbation theory on the Thiel set
Source: arXiv:2302.07240 source file (2023-05-20)
Supplement: Supplementary file 48 [file pyrazine_vs_TBE_errors.tex]

\begin{table}[htp]
\caption{ 
\label{tab:pyrazine_ESMP2_vs_TBE}
Absolute ESMF, ESMP2 and level shifted ESMP2 (level shift = 0.50 a.u.) results vs. the Thiel best estimates (TBEs) for pyrazine.}
\begin{tabular}{l| c | c c | c c | c c}
\hline\hline
\hspace{2mm} State & 
\hspace{2mm} TBE & 
\hspace{2mm} ESMF & 
\hspace{2mm} error & 
\hspace{2mm} ESMP2 & 
\hspace{2mm} error & 
\hspace{2mm} shift=0.50 a.u. & 
\hspace{2mm} error 
\\[2pt] 
\hline 
\hspace{0.0mm} $1^1B_{3u}$ & 3.95 & 4.94 & 0.99 & 3.34 & 0.61 & 4.00 & 0.05 \\ 
\hspace{0.0mm} $1^1A_{u}$ & 4.81 & 6.61 & 1.80 & 3.84 & 0.97 & 4.81 & 0.00 \\ 
\hspace{0.0mm} $1^1B_{2u}$ & 4.64 & 5.57 & 0.93 & 4.25 & 0.39 & 4.86 & 0.22 \\ 
\hspace{0.0mm} $1^1B_{2g}$ & 5.56 & 6.38 & 0.82 & 4.92 & 0.64 & 5.65 & 0.09 \\ 
\hspace{0.0mm} $1^1B_{1g}$ & 6.60 & 8.71 & 2.11 & 5.42 & 1.18 & 6.69 & 0.09 \\ 
\hspace{0.0mm} $1^1B_{1u}$ & 6.58 & 6.63 & 0.05 & 6.48 & 0.10 & 6.66 & 0.08 \\ 
\hspace{0.0mm} $2^1B_{1u}$ & 7.72 & 8.54 & 0.82 & 6.91 & 0.81 & 7.62 & 0.10 \\ 
\hspace{0.0mm} $2^1B_{2u}$ & 7.60 & 8.64 & 1.04 & 6.99 & 0.61 & 7.76 & 0.16 \\ 
\hline\hline 
\end{tabular} 
\end{table}
