# Supplementary material for: Studying excited-state-specific perturbation theory on the Thiel set
Source: arXiv:2302.07240 source file (2023-05-20)
Supplement: Supplementary file 49 [file pyridazine_vs_TBE_errors.tex]

\begin{table}[htp]
\caption{ 
\label{tab:pyridazine_ESMP2_vs_TBE}
Absolute ESMF, ESMP2 and level shifted ESMP2 (level shift = 0.50 a.u.) results vs. the Thiel best estimates (TBEs) for pyridazine.}
\begin{tabular}{l| c | c c | c c | c c}
\hline\hline
\hspace{2mm} State & 
\hspace{2mm} TBE & 
\hspace{2mm} ESMF & 
\hspace{2mm} error & 
\hspace{2mm} ESMP2 & 
\hspace{2mm} error & 
\hspace{2mm} shift=0.50 a.u. & 
\hspace{2mm} error 
\\[2pt] 
\hline 
\hspace{0.0mm} $1^1B_{1}$ & 3.78 & 4.33 & 0.55 & 3.26 & 0.52 & 3.67 & 0.11 \\ 
\hspace{0.0mm} $1^1A_{2}$ & 4.32 & 5.18 & 0.86 & 3.66 & 0.66 & 4.25 & 0.07 \\ 
\hspace{0.0mm} $2^1A_{1}$ & 5.18 & 6.20 & 1.02 & 4.28 & 0.90 & 5.16 & 0.02 \\ 
\hspace{0.0mm} $2^1A_{2}$ & 5.77 & 6.54 & 0.77 & 4.82 & 0.95 & 5.53 & 0.24 \\ 
\hline\hline 
\end{tabular} 
\end{table}
