# Supplementary material for: Studying excited-state-specific perturbation theory on the Thiel set
Source: arXiv:2302.07240 source file (2023-05-20)
Supplement: Supplementary file 50 [file pyridine_vs_TBE_errors.tex]

\begin{table}[htp]
\caption{ 
\label{tab:pyridine_ESMP2_vs_TBE}
Absolute ESMF, ESMP2 and level shifted ESMP2 (level shift = 0.50 a.u.) results vs. the Thiel best estimates (TBEs) for pyridine.}
\begin{tabular}{l| c | c c | c c | c c}
\hline\hline
\hspace{2mm} State & 
\hspace{2mm} TBE & 
\hspace{2mm} ESMF & 
\hspace{2mm} error & 
\hspace{2mm} ESMP2 & 
\hspace{2mm} error & 
\hspace{2mm} shift=0.50 a.u. & 
\hspace{2mm} error 
\\[2pt] 
\hline 
\hspace{0.0mm} $1^1B_{2}$ & 4.85 & 5.97 & 1.12 & 4.52 & 0.33 & 5.19 & 0.34 \\ 
\hspace{0.0mm} $1^1B_{1}$ & 4.59 & 4.70 & 0.11 & 4.93 & 0.34 & 4.98 & 0.39 \\ 
\hspace{0.0mm} $2^1A_{2}$ & 5.11 & 5.65 & 0.54 & 5.25 & 0.14 & 5.50 & 0.39 \\ 
\hspace{0.0mm} $2^1A_{1}$ & 6.26 & 6.47 & 0.21 & 6.22 & 0.04 & 6.45 & 0.19 \\ 
\hspace{0.0mm} $3^1A_{1}$ & 7.18 & 8.21 & 1.03 & 6.55 & 0.63 & 7.29 & 0.11 \\ 
\hspace{0.0mm} $2^1B_{2}$ & 7.27 & 8.14 & 0.87 & 6.54 & 0.73 & 7.25 & 0.02 \\ 
\hline\hline 
\end{tabular} 
\end{table}
