# Supplementary material for: Studying excited-state-specific perturbation theory on the Thiel set
Source: arXiv:2302.07240 source file (2023-05-20)
Supplement: Supplementary file 51 [file pyrimidine_vs_TBE_errors.tex]

\begin{table}[htp]
\caption{ 
\label{tab:pyrimidine_ESMP2_vs_TBE}
Absolute ESMF, ESMP2 and level shifted ESMP2 (level shift = 0.50 a.u.) results vs. the Thiel best estimates (TBEs) for pyrimidine.}
\begin{tabular}{l| c | c c | c c | c c}
\hline\hline
\hspace{2mm} State & 
\hspace{2mm} TBE & 
\hspace{2mm} ESMF & 
\hspace{2mm} error & 
\hspace{2mm} ESMP2 & 
\hspace{2mm} error & 
\hspace{2mm} shift=0.50 a.u. & 
\hspace{2mm} error 
\\[2pt] 
\hline 
\hspace{0.0mm} $1^1B_{1}$ & 4.55 & 5.17 & 0.62 & 3.65 & 0.90 & 4.24 & 0.31 \\ 
\hspace{0.0mm} $1^1A_{2}$ & 4.91 & 5.89 & 0.98 & 4.18 & 0.73 & 4.83 & 0.08 \\ 
\hspace{0.0mm} $1^1B_{2}$ & 5.44 & 6.20 & 0.76 & 4.96 & 0.48 & 5.55 & 0.11 \\ 
\hspace{0.0mm} $2^1A_{1}$ & 6.95 & 8.31 & 1.36 & 6.36 & 0.59 & 7.25 & 0.30 \\ 
\hline\hline 
\end{tabular} 
\end{table}
