# Supplementary material for: Studying excited-state-specific perturbation theory on the Thiel set
Source: arXiv:2302.07240 source file (2023-05-20)
Supplement: Supplementary file 53 [file tetrazine_vs_TBE_errors.tex]

\begin{table}[htp]
\caption{ 
\label{tab:tetrazine_ESMP2_vs_TBE}
Absolute ESMF, ESMP2 and level shifted ESMP2 (level shift = 0.50 a.u.) results vs. the Thiel best estimates (TBEs) for tetrazine.}
\begin{tabular}{l| c | c c | c c | c c}
\hline\hline
\hspace{2mm} State & 
\hspace{2mm} TBE & 
\hspace{2mm} ESMF & 
\hspace{2mm} error & 
\hspace{2mm} ESMP2 & 
\hspace{2mm} error & 
\hspace{2mm} shift=0.50 a.u. & 
\hspace{2mm} error 
\\[2pt] 
\hline 
\hspace{0.0mm} $1^1B_{3u}$ & 2.24 & 3.34 & 1.10 & 1.36 & 0.88 & 2.12 & 0.12 \\ 
\hspace{0.0mm} $1^1A_{u}$ & 3.48 & 5.39 & 1.91 & 2.48 & 1.00 & 3.55 & 0.07 \\ 
\hspace{0.0mm} $1^1B_{1g}$ & 4.73 & 5.99 & 1.26 & 4.06 & 0.67 & 4.94 & 0.21 \\ 
\hspace{0.0mm} $1^1B_{2u}$ & 4.91 & 5.96 & 1.05 & 3.98 & 0.93 & 4.86 & 0.05 \\ 
\hspace{0.0mm} $2^1A_{u}$ & 5.47 & 6.53 & 1.06 & 3.61 & 1.86 & 4.75 & 0.72 \\ 
\hspace{0.0mm} $1^1B_{2g}$ & 5.18 & 6.41 & 1.23 & 4.25 & 0.93 & 5.28 & 0.10 \\ 
\hline\hline 
\end{tabular} 
\end{table}
