# Supplementary material for: Studying excited-state-specific perturbation theory on the Thiel set
Source: arXiv:2302.07240 source file (2023-05-20)
Supplement: Supplementary file 54 [file thymine_vs_TBE_errors.tex]

\begin{table}[htp]
\caption{ 
\label{tab:thymine_ESMP2_vs_TBE}
Absolute ESMF, ESMP2 and level shifted ESMP2 (level shift = 0.50 a.u.) results vs. the Thiel best estimates (TBEs) for thymine.}
\begin{tabular}{l| c | c c | c c | c c}
\hline\hline
\hspace{2mm} State & 
\hspace{2mm} TBE & 
\hspace{2mm} ESMF & 
\hspace{2mm} error & 
\hspace{2mm} ESMP2 & 
\hspace{2mm} error & 
\hspace{2mm} shift=0.50 a.u. & 
\hspace{2mm} error 
\\[2pt] 
\hline 
\hspace{0.0mm} $1^1A^{\prime\prime}$ & 4.82 & 4.26 & 0.56 & 4.91 & 0.09 & 4.90 & 0.08 \\ 
\hspace{0.0mm} $2^1A'$ & 5.20 & 5.96 & 0.76 & 4.84 & 0.36 & 5.29 & 0.09 \\ 
\hspace{0.0mm} $3^1A'$ & 6.27 & 7.50 & 1.23 & 4.56 & 1.71 & 5.94 & 0.33 \\ 
\hspace{0.0mm} $2^1A^{\prime\prime}$ & 6.16 & 5.62 & 0.54 & 6.55 & 0.39 & 6.44 & 0.28 \\ 
\hspace{0.0mm} $4^1A'$ & 6.53 & 8.68 & 2.15 & 4.91 & 1.62 & 6.45 & 0.08 \\ 
\hline\hline 
\end{tabular} 
\end{table}
