# Supplementary material for: Studying excited-state-specific perturbation theory on the Thiel set
Source: arXiv:2302.07240 source file (2023-05-20)
Supplement: Supplementary file 55 [file triazine_vs_TBE_errors.tex]

\begin{table}[htp]
\caption{ 
\label{tab:triazine_ESMP2_vs_TBE}
Absolute ESMF, ESMP2 and level shifted ESMP2 (level shift = 0.50 a.u.) results vs. the Thiel best estimates (TBEs) for triazine.}
\begin{tabular}{l| c | c c | c c | c c}
\hline\hline
\hspace{2mm} State & 
\hspace{2mm} TBE & 
\hspace{2mm} ESMF & 
\hspace{2mm} error & 
\hspace{2mm} ESMP2 & 
\hspace{2mm} error & 
\hspace{2mm} shift=0.50 a.u. & 
\hspace{2mm} error 
\\[2pt] 
\hline 
\hspace{0.0mm} $1^1A_{1}^{\prime\prime}$ & 4.60 & 6.04 & 1.44 & 3.23 & 1.37 & 4.44 & 0.16 \\ 
\hspace{0.0mm} $1^1A_{2}^{\prime\prime}$ & 4.66 & 6.14 & 1.48 & 3.65 & 1.01 & 4.48 & 0.18 \\ 
\hspace{0.0mm} $1^1E^{\prime\prime}$ & 4.71 & 6.16 & 1.45 & 3.49 & 1.22 & 4.48 & 0.23 \\ 
\hspace{0.0mm} $1^1A_2^\prime$ & 5.79 & 6.95 & 1.16 & 4.34 & 1.45 & 5.48 & 0.31 \\ 
\hline\hline 
\end{tabular} 
\end{table}
