# Supplementary material for: Studying excited-state-specific perturbation theory on the Thiel set
Source: arXiv:2302.07240 source file (2023-05-20)
Supplement: Supplementary file 56 [file uracil_vs_TBE_errors.tex]

\begin{table}[htp]
\caption{ 
\label{tab:uracil_ESMP2_vs_TBE}
Absolute ESMF, ESMP2 and level shifted ESMP2 (level shift = 0.50 a.u.) results vs. the Thiel best estimates (TBEs) for uracil.}
\begin{tabular}{l| c | c c | c c | c c}
\hline\hline
\hspace{2mm} State & 
\hspace{2mm} TBE & 
\hspace{2mm} ESMF & 
\hspace{2mm} error & 
\hspace{2mm} ESMP2 & 
\hspace{2mm} error & 
\hspace{2mm} shift=0.50 a.u. & 
\hspace{2mm} error 
\\[2pt] 
\hline 
\hspace{0.0mm} $1^1A^{\prime\prime}$ & 4.80 & 4.24 & 0.56 & 4.82 & 0.02 & 4.83 & 0.03 \\ 
\hspace{0.0mm} $2^1A'$ & 5.35 & 6.18 & 0.83 & 4.80 & 0.55 & 5.36 & 0.01 \\ 
\hspace{0.0mm} $3^1A^{\prime\prime}$ & 6.56 & 8.98 & 2.42 & 5.63 & 0.93 & 6.93 & 0.37 \\ 
\hspace{0.0mm} $2^1A^{\prime\prime}$ & 6.10 & 5.56 & 0.54 & 6.49 & 0.39 & 6.39 & 0.29 \\ 
\hspace{0.0mm} $4^1A'$ & 6.70 & 8.12 & 1.42 & 5.14 & 1.56 & 6.40 & 0.30 \\ 
\hline\hline 
\end{tabular} 
\end{table}
